# Supplementary material for: DOCTOR: A Simple Method for Detecting Misclassification Errors
Source: arXiv:2106.02395 source file (2021-10-29)
Supplement: Supplementary file 1 [file mahalanobis.tex]

\newpage
\section{Mahalanobis}
\begin{table}[!htb]
	\caption{Best AUROCs obtained via DOCTOR, ODIN and SR and Mahalanobis for image datasets. Values in bold correspond to the maximum AUROCs. MHLNB$_1$ denotes Mahalanobis as in~\eqref{eq:mhlnb} whilst MHLNB$_2$ is~\eqref{eq:mhlnb} by using logits in place of softmax output.}
	\begin{center}
		\begin{small}
			\resizebox{.36\textwidth}{!}{
			\begin{sc}
				\begin{tabular}{c|c|c}
				    \toprule
					\textbf{DATASET} & \textbf{METHOD} & \textbf{AUROC $\%$}\\ 
					\hline
					\midrule
					\multirow{5}{*}{\parbox[t][][c]{3cm}{\centering
 CIFAR10\\\textnormal{Accuracy} $95\%$}}  & $D_\alpha$ & \textbf{94.3} \\ \cmidrule{2-3}
& ODIN       & 87.4\\\cmidrule{2-3}
& SR         & 93.8\\\cmidrule{2-3}
& MHLNB$_{1}$  & 94\\\cmidrule{2-3}
& MHLNB$_{2}$  & 84.2\\
\midrule
				    \multirow{5}{*}{\parbox[t][][c]{3cm}{\centering
 CIFAR100\\\textnormal{Accuracy} $78\%$}} & $D_\alpha$ & \textbf{87}\\\cmidrule{2-3}
& ODIN       &  78\\ \cmidrule{2-3}
& SR         &  86.9\\\cmidrule{2-3}
& MHLNB$_{1}$  & 82.6\\\cmidrule{2-3}
& MHLNB$_{2}$  & 50\\
\midrule
					\multirow{5}{*}{\parbox[t][][c]{3cm}{\centering
 TinyImageNet\\\textnormal{Accuracy} $63\%$}}   & $D_\alpha$ & \textbf{84.9}\\\cmidrule{2-3}
& ODIN       & 78.8\\ \cmidrule{2-3}
& SR         & \textbf{84.9} \\\cmidrule{2-3}
& MHLNB$_{1}$  & 78.4\\\cmidrule{2-3}
& MHLNB$_{2}$  & 59\\
\midrule
					\multirow{3}{*}{\parbox[t][][c]{3cm}{\centering
 SVHN\\ \textnormal{Accuracy} $96\%$}} & $D_\alpha$ & \textbf{92.3}\\\cmidrule{2-3}
& ODIN       & 89.1\\ \cmidrule{2-3}
& SR         & \textbf{92.3}\\\cmidrule{2-3}
& MHLNB  & 87.4\\\cmidrule{2-3}
& MHLNB$_{l}$  & 87.9\\
\bottomrule
				    \end{tabular}
			    \end{sc}
		    }
	    \end{small}
    \end{center}
\label{tab:best_aurocs_mahalanobis}
\end{table}
Recall from \cref{sec:preliminaries}, $\mathcal{D}_n=\{(\mathbf{x}_1, y_1),\dots,(\mathbf{x}_n, y_n)\}\sim p_{XY}$ is the training set, where $\mathbf{x}_i\in\mathcal{X}$ is the input sample, $y_i\in\{1,\dots,C\}$ is the true class of $\mathbf{x}_i$ among $C$ possible classes and $n$ denotes the size of the training set. Moreover, for brevity let us set $f(\mathbf{x})\equiv f_{\mathcal{D}_n}(\mathbf{x})$.
We define the \textit{empirical mean}, the \textit{empirical class mean} and the \textit{empirical covariance} of training samples as follows:
\begin{align}
    %\widehat{\mu} &\myeq \frac{1}{n} \sum_{i=1}^n f(\mathbf{x}_i)\\
    \widehat{\mu}_c &\myeq \frac{1}{n_c} \sum_{i:y_i=c} f(\mathbf{x}_i)\\
    \widehat{\Sigma} &\myeq \frac{1}{n}\sum_c \sum_{i:y_i=c} (f(\mathbf{x}_i) - \widehat{\mu}_c)(f(\mathbf{x}_i) - \widehat{\mu}_c)^\top,
\end{align}
where $n_c$ is the number of training samples with label $c$.% and $f_{-1}$ denotes the logits.
\begin{definition}[MHLNB]
For any $\mathbf{x}\in\mathcal{X}$, let $c$ be its predicted class. By MHLNB we denote, respectively:
\begin{align}\label{eq:mhlnb}
    M(\mathbf{x}) &\myeq \max\limits_{c}~-(f(\mathbf{x}) - \widehat{\mu}_c)^\top\cdot\widehat{\Sigma}^{-1}\cdot (f(\mathbf{x}) - \widehat{\mu}_c).
\end{align}
\end{definition}
\section{Normalization}
\subsection{Norm by max-sum}
Probabilities as in email and then DOCTOR in its pure form.
\begin{itemize}
    \item CIFAR10: 93.5
    \item CIFAR100: 82.7
    \item TinyImageNet: 84
    \item SVHN: 91.1
\end{itemize}
\subsection{Weighted norm}
Use the vector of before as vector of weights for softmax. Put weight of the predicted class to 1.
\begin{itemize}
    \item CIFAR10: 94.18
    \item CIFAR100: 86.9
    \item TinyImageNet: 84.9
    \item SVHN: 92.3
\end{itemize}
\subsection{$0$-norm}
Compute:
\begin{align*}
    P(\mathbf{x}) = \frac{1}{n_{classes}}\sum_i\mathbf{1}[l_i(\mathbf{x})>\gamma]
\end{align*}
\begin{itemize}
    \item CIFAR10: 
    \item CIFAR100: 
    \item TinyImageNet: 
    \item SVHN: 
\end{itemize}
\section{MNIST with bad classifier}
Accuracy : $30\%$
\includegraphics[scale=0.5]{figures/plots/mnist_best_T_1_2.png}
\section{Perturbation}
$T = 1$, $\epsilon = 0.003$. No validation set.
\subsection{D$_\alpha$}
\begin{equation}
    L_\alpha(\mathbf{x}) = -\log(1 - \fun{g}(\mathbf{x})) + \log(\fun{g}(\mathbf{x}))
\end{equation}
\begin{itemize}
    \item CIFAR10: 95.32
    \item CIFAR100: 88.2
    \item TinyImageNet: 85.78
    \item SVHN: 92.7
\end{itemize}
\subsection{D$_\beta$}
\begin{equation*}
    L_\beta(\mathbf{x}, f(\mathbf{x})) = -\log(1 - P_{\widehat{Y}|X}(f(\mathbf{x}) |\mathbf{x})) + \log(P_{\widehat{Y}|X}(f(\mathbf{x}) |\mathbf{x}))
\end{equation*}
\begin{itemize}
    \item CIFAR10: 94.9 
    \item CIFAR100: 84.9
    \item TinyImageNet: 85.7
    \item SVHN: 92.7
\end{itemize}
\section{Simulation on perturbation}
\subsection{Simulation by varying $T$ and $\epsilon$}

\begin{figure}[!htb]
	\centering
	\begin{subfigure}[b]{0.23\textwidth}
	    \centering
x	    \includegraphics[width=\textwidth]{figures/plots/cifar10_eps_auroc.png}
	    \vspace{-1.5\baselineskip}
	    \caption{CIFAR10: $T=1$}
	    \label{fig:cifar10_best_eps}
	\end{subfigure}
	\begin{subfigure}[b]{0.23\textwidth}
	    \centering
x	    \includegraphics[width=\textwidth]{figures/plots/cifar100_eps_auroc.png}
	    \vspace{-1.5\baselineskip}
	    \caption{CIFAR100: $T=1$}
	    \label{fig:cifar100_best_eps}
	\end{subfigure}
	\begin{subfigure}[b]{0.23\textwidth}
	    \centering
	    \includegraphics[width=\textwidth]{figures/plots/tinyimagenet_best_eps.png}
	    \vspace{-1.5\baselineskip}
	    \caption{TinyImageNet: $T=1$}
	    \label{fig:tiny_best_eps}
	\end{subfigure}
	\begin{subfigure}[b]{0.23\textwidth}
	    \centering
	    \includegraphics[width=\textwidth]{figures/plots/svhn_best_eps.png}
	    \vspace{-1.5\baselineskip}
	    \caption{SVHN: $T=1$}
	    \label{fig:svhn_best_eps}
	\end{subfigure}
	\caption{AUROCs obtained via $D_\alpha$ according to the best value of $T$ and by varying $\epsilon$ as in~\cref{tab:best_eps_alpha}.}
	\label{fig:auc}
\end{figure}

x \subsection{Table summarising all results}
\begin{table}[!htb]
	\caption{Best AUROCs obtained via DOCTOR, ODIN and SR and Mahalanobis for image datasets. Values in bold correspond to the maximum AUROCs. In \textit{totally black box} only the last layer of the network is available, hence no input pre-processing can be performed. In \textit{partially black box} we suppose is possible to perturb the input as in~\cref{eq:perturb_alpha},~\cref{eq:perturb_odin} and~\cref{eq:perturb_mahalanobis} for $D_\alpha$, ODIN and MHLNB, respectively. The perturbation values are: $\epsilon_{\alpha}=0.0035$ for $D_\alpha$; $\epsilon_{\text{ODIN}}$ as in \cite{LiangLS2018ICLR} for ODIN; $\epsilon_{\text{MHLNB}}=$ for MHLNB.}
	\begin{center}
		\begin{small}
			\resizebox{.7\textwidth}{!}{
			\begin{sc}
				\begin{tabular}{c|c|c|c}
				    \toprule
					\textbf{DATASET} & \textbf{DISCRIMINATOR} & \textbf{AUROC $\%$} & \textbf{AUROC $\%$}\\
					 &  & totally black box & partially black box\\ 
					\hline
					\midrule
					\multirow{4}{*}{\parbox[t][][c]{3cm}{\centering
 CIFAR10\\\textnormal{Accuracy} $95\%$}}  & $D_\alpha$ & \textbf{94.3} & \textbf{95.2} \\ \cmidrule{2-4}
& ODIN       & - & 87.4\\\cmidrule{2-4}
& SR         & 93.8 & -\\\cmidrule{2-4}
& MHLNB  & 84.2 & \\
\midrule
				    \multirow{4}{*}{\parbox[t][][c]{3cm}{\centering
 CIFAR100\\\textnormal{Accuracy} $78\%$}} & $D_\alpha$ & \textbf{87} & \textbf{88.2}\\\cmidrule{2-4}
& ODIN       & - & 78\\ \cmidrule{2-4}
& SR         &  86.9 & -\\\cmidrule{2-4}
& MHLNB  & 50 &\\
\midrule
					\multirow{4}{*}{\parbox[t][][c]{3cm}{\centering
 TinyImageNet\\\textnormal{Accuracy} $63\%$}}   & $D_\alpha$ & \textbf{84.9} & \textbf{86}\\\cmidrule{2-4}
& ODIN       & - & 78.8\\ \cmidrule{2-4}
& SR         & \textbf{84.9} & - \\\cmidrule{2-4}
& MHLNB  & 59 &\\
\midrule
					\multirow{4}{*}{\parbox[t][][c]{3cm}{\centering
 SVHN\\ \textnormal{Accuracy} $96\%$}} & $D_\alpha$ & \textbf{92.3} & \textbf{93}\\\cmidrule{2-4}
& ODIN       & - & 89.1\\ \cmidrule{2-4}
& SR         & \textbf{92.3} & -\\\cmidrule{2-4}
& MHLNB  & 87.9 &\\
\bottomrule
				    \end{tabular}
			    \end{sc}
		    }
	    \end{small}
    \end{center}
\label{tab:best_aurocs_total}
\end{table}

% \begin{definition}[Perturbation ODIN~\cite{LiangLS2018ICLR}]
% \begin{align}\label{eq:perturb_odin}
%     \widetilde{\mathbf{x}} = \mathbf{x} - \epsilon\text{sign}(-\nabla_{\mathbf{x}}\log(\text{SODIN}(\mathbf{x})))
% \end{align}
% \end{definition}
% \begin{definition}[Perturbation DOCTOR]
% \begin{align}
%     \widetilde{\mathbf{x}} = \mathbf{x} + \epsilon\text{sign}(\nabla_{\mathbf{x}}-\log (\ghat(\mathbf{x})) + \log(\gh(\mathbf{x})))
% \end{align}
% \begin{align}
%     \widetilde{\mathbf{x}} = \mathbf{x} + \epsilon\text{sign}(\nabla_{\mathbf{x}}-\log (\pehat(\mathbf{x})) + \log(1 - \pehat(\mathbf{x})))
% \end{align}
% \end{definition}
% \begin{definition}[Perturbation Mahalanobis~\cite{LeeLLS2018NeurIPS}]
% \begin{align}\label{eq:perturb_mahalanobis}
%     \widetilde{\mathbf{x}} = \mathbf{x} + \epsilon\text{sign}(\nabla_{\mathbf{x}}M(\mathbf{x}))
% \end{align}
% \end{definition}
